# Supplementary material for: A Multi-faceted Analysis of the Performance Variability of Virtual Machines
Source: arXiv:2309.11959 source file (2023-09-21)
Supplement: Supplementary file 1 [file appendix.tex]

\nw{In this appendix, we first show the correlation matrices between resource metrics for Azure and EGI (Figure~\ref{fig:correlation2}), then in Table~\ref{tab:forecasting-var} and Table~\ref{tab:forecasting-sarimax} we present the detailed results of time-series forecasting with respect to the VAR and SARIMAX models respectively.}

\begin{figure}[ht]
	\centering
	\includegraphics[width=0.75\linewidth]{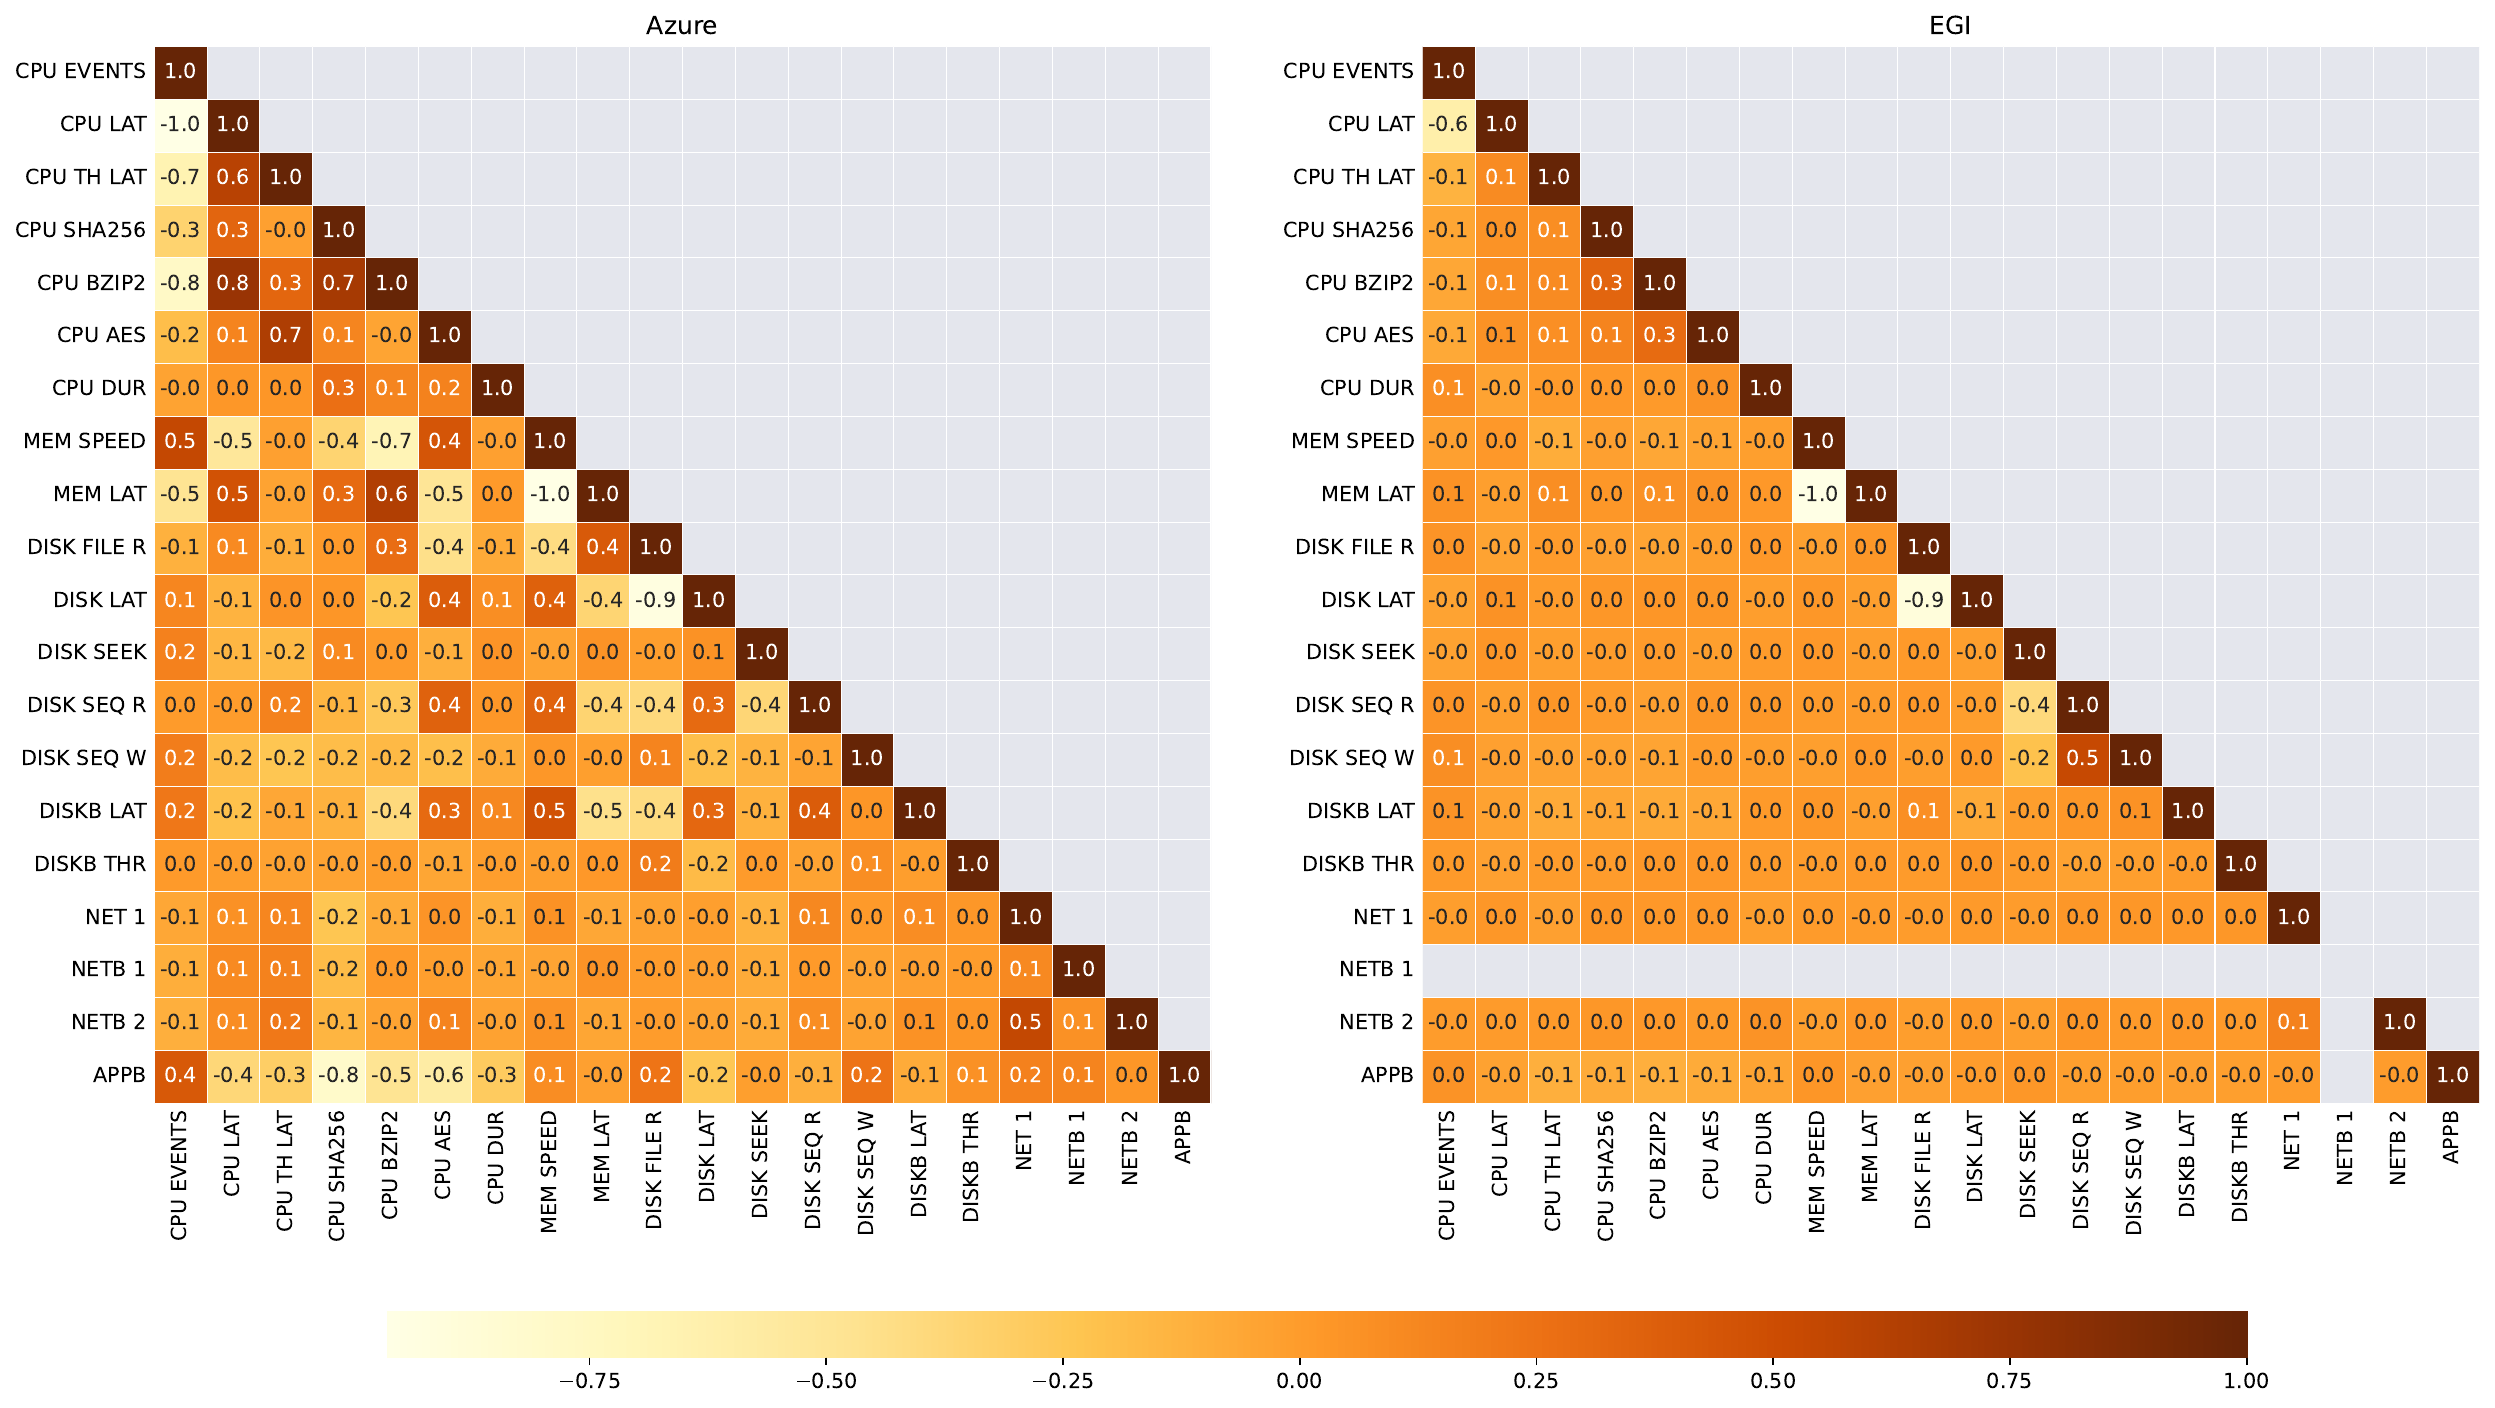}
	\caption{\nw{Correlation between resource metrics for Azure and EGI.}}
	\label{fig:correlation2}
\end{figure}

\begin{table*}[ht]

\setlength{\tabcolsep}{3.4pt}
\fontsize{8}{9.6}\selectfont
\centering
\begin{tabular}{@{}r|cccc|cccc|cccc|cccc|c@{}}
& \multicolumn{4}{c|}{\textbf{AWS}} & \multicolumn{4}{c|}{\textbf{Azure}} & \multicolumn{4}{c|}{\textbf{GCP}} & \multicolumn{4}{c|}{\textbf{EGI}} & \\ \hline
\textbf{Metric} & C1 & C2 & C3 & C4 & C1 & C2 & C3 & C4 & C1 & C2 & C3 & C4 & C1 & C2 & C3 & C4 & \textbf{Overall} \\ \hline
CPU EVENTS & 0.62 \phantom{-} & 1.02 \phantom{-} & 1.01 \textsuperscript{\textdagger} & 0.63 \textsuperscript{\textdagger} & 1.55 \phantom{-} & 1.06 \phantom{-} & 0.28 \textsuperscript{\textdagger} & 1.27 \phantom{-} & 1.37 \phantom{-} & 0.47 \textsuperscript{\textdagger} & 1.30 \phantom{-} & 0.39 \textsuperscript{\textdagger} & 0.56 \textsuperscript{\textdagger} & 0.76 \phantom{-} & 0.76 \phantom{-} & 1.31 \phantom{-} & 0.9 \\
CPU LAT & 0.67 \phantom{-} & 0.97 \phantom{-} & 1.17 \phantom{-} & 0.80 \phantom{-} & 1.35 \phantom{-} & 1.22 \phantom{-} & 0.37 \textsuperscript{\textdagger} & 1.46 \phantom{-} & 0.75 \phantom{-} & 1.36 \textsuperscript{\textdagger} & 0.92 \phantom{-} & 0.86 \textsuperscript{\textdagger} & 1.03 \phantom{-} & 1.80 \textsuperscript{\textdaggerdbl} & 1.00 \phantom{-} & 4.25 \phantom{-} & 1.25 \\
CPU TH LAT & 0.60 \textsuperscript{\textdagger} & 0.71 \textsuperscript{\textdagger} & 0.69 \phantom{-} & 0.97 \phantom{-} & 1.44 \phantom{-} & 0.96 \phantom{-} & 0.94 \phantom{-} & 1.88 \phantom{-} & 1.49 \phantom{-} & 0.95 \phantom{-} & 0.68 \textsuperscript{\textdagger} & 0.73 \phantom{-} & 0.44 \textsuperscript{\textdagger} & 0.95 \phantom{-} & 0.67 \phantom{-} & 0.84 \phantom{-} & 0.93 \\
CPU SHA256 & 1.58 \phantom{-} & 0.38 \textsuperscript{\textdagger} & 0.80 \textsuperscript{\textdagger} & 0.54 \textsuperscript{\textdaggerdbl} & 1.91 \phantom{-} & 1.06 \phantom{-} & 0.40 \textsuperscript{\textdagger} & 1.67 \phantom{-} & 1.35 \phantom{-} & 0.52 \phantom{-} & 0.48 \phantom{-} & 0.89 \phantom{-} & 1.07 \phantom{-} & 1.05 \phantom{-} & 0.74 \phantom{-} & 0.87 \phantom{-} & 0.96 \\
CPU BZIP2 & 1.28 \phantom{-} & 0.72 \phantom{-} & 1.28 \textsuperscript{\textdaggerdbl} & 0.49 \textsuperscript{\textdagger} & 1.96 \phantom{-} & 1.60 \phantom{-} & 0.40 \textsuperscript{\textdagger} & 2.31 \phantom{-} & 0.69 \phantom{-} & 0.71 \phantom{-} & 0.81 \phantom{-} & 0.72 \phantom{-} & 1.04 \phantom{-} & 1.12 \phantom{-} & 1.10 \phantom{-} & 1.03 \phantom{-} & 1.08 \\
CPU AES & 2.76 \phantom{-} & 0.65 \textsuperscript{\textdagger} & 0.66 \textsuperscript{\textdagger} & 0.70 \textsuperscript{\textdagger} & 1.47 \phantom{-} & 1.97 \phantom{-} & 1.07 \phantom{-} & 2.26 \phantom{-} & 0.51 \textsuperscript{\textdagger} & 1.14 \phantom{-} & 0.70 \textsuperscript{\textdagger} & 0.76 \textsuperscript{\textdagger} & 0.59 \phantom{-} & 1.03 \phantom{-} & 0.57 \phantom{-} & 1.19 \phantom{-} & 1.13 \\
CPU DUR & 1.15 \phantom{-} & 0.92 \phantom{-} & 0.73 \phantom{-} & 1.07 \phantom{-} & 1.15 \phantom{-} & 0.88 \phantom{-} & 0.92 \phantom{-} & 1.50 \phantom{-} & 0.86 \phantom{-} & 0.57 \phantom{-} & 0.98 \phantom{-} & 0.82 \phantom{-} & 0.79 \phantom{-} & 0.66 \phantom{-} & 1.12 \phantom{-} & 0.75 \phantom{-} & 0.93 \\
MEM SPEED & 0.96 \textsuperscript{\textdagger} & 0.58 \textsuperscript{\textdagger} & 0.34 \textsuperscript{\textdaggerdbl} & 0.77 \phantom{-} & 2.01 \phantom{-} & 1.85 \phantom{-} & 1.02 \phantom{-} & 1.26 \phantom{-} & 0.44 \textsuperscript{\textdaggerdbl} & 0.63 \textsuperscript{\textdagger} & 0.52 \textsuperscript{\textdaggerdbl} & 0.96 \phantom{-} & 0.53 \phantom{-} & 0.92 \phantom{-} & 0.91 \phantom{-} & 0.43 \phantom{-} & 0.88 \\
MEM LAT & 1.02 \textsuperscript{\textdagger} & 0.85 \textsuperscript{\textdagger} & 0.30 \textsuperscript{\textdaggerdbl} & 0.57 \phantom{-} & 2.09 \phantom{-} & 1.93 \phantom{-} & 1.16 \phantom{-} & 0.84 \phantom{-} & 0.77 \textsuperscript{\textdaggerdbl} & 0.99 \phantom{-} & 0.47 \textsuperscript{\textdaggerdbl} & 1.05 \phantom{-} & 0.56 \phantom{-} & 0.98 \phantom{-} & 0.86 \phantom{-} & 0.34 \textsuperscript{\textdagger} & 0.92 \\
DISK FILE R & 0.71 \phantom{-} & 0.48 \phantom{-} & 0.76 \phantom{-} & 0.42 \phantom{-} & 1.92 \phantom{-} & 1.79 \phantom{-} & 3.76 \phantom{-} & 4.61 \phantom{-} & 0.62 \phantom{-} & 0.54 \phantom{-} & 1.36 \phantom{-} & 0.43 \phantom{-} & 0.74 \phantom{-} & 1.46 \phantom{-} & 0.87 \phantom{-} & 0.51 \phantom{-} & 1.31 \\
DISK FILE W & 0.71 \phantom{-} & 0.48 \phantom{-} & 0.76 \phantom{-} & 0.42 \phantom{-} & 1.92 \phantom{-} & 1.79 \phantom{-} & 3.76 \phantom{-} & 4.61 \phantom{-} & 0.62 \phantom{-} & 0.54 \phantom{-} & 1.36 \phantom{-} & 0.43 \phantom{-} & 0.74 \phantom{-} & 1.46 \phantom{-} & 0.87 \phantom{-} & 0.51 \phantom{-} & 1.31 \\
DISK FILE F & 0.71 \phantom{-} & 0.48 \phantom{-} & 0.76 \phantom{-} & 0.42 \phantom{-} & 1.92 \phantom{-} & 1.79 \phantom{-} & 3.75 \phantom{-} & 4.61 \phantom{-} & 0.62 \phantom{-} & 0.55 \phantom{-} & 1.36 \phantom{-} & 0.43 \phantom{-} & 0.69 \phantom{-} & 1.46 \phantom{-} & 0.87 \phantom{-} & 0.51 \phantom{-} & 1.31 \\
DISK THR R & 0.71 \phantom{-} & 0.48 \phantom{-} & 0.76 \phantom{-} & 0.42 \phantom{-} & 1.92 \phantom{-} & 1.79 \phantom{-} & 3.76 \phantom{-} & 4.61 \phantom{-} & 0.62 \phantom{-} & 0.55 \phantom{-} & 1.36 \phantom{-} & 0.43 \phantom{-} & 0.75 \phantom{-} & 1.46 \phantom{-} & 0.87 \phantom{-} & 0.51 \phantom{-} & 1.31 \\
DISK THR W & 0.71 \phantom{-} & 0.48 \phantom{-} & 0.76 \phantom{-} & 0.42 \phantom{-} & 1.92 \phantom{-} & 1.79 \phantom{-} & 3.76 \phantom{-} & 4.61 \phantom{-} & 0.62 \phantom{-} & 0.55 \phantom{-} & 1.36 \phantom{-} & 0.43 \phantom{-} & 0.72 \phantom{-} & 1.47 \phantom{-} & 0.86 \phantom{-} & 0.51 \phantom{-} & 1.31 \\
DISK LAT & 1.27 \phantom{-} & 0.20 \textsuperscript{\textdaggerdbl} & 1.09 \phantom{-} & 0.27 \phantom{-} & 1.43 \phantom{-} & 1.28 \phantom{-} & 4.13 \phantom{-} & 5.57 \phantom{-} & 0.56 \phantom{-} & 0.57 \phantom{-} & 1.39 \phantom{-} & 0.52 \phantom{-} & 0.77 \textsuperscript{\textdagger} & 1.60 \phantom{-} & 0.56 \phantom{-} & 0.72 \phantom{-} & 1.37 \\
DISK SEEK & -- & -- & 1.56 \textsuperscript{\textdaggerdbl} & 0.81 \textsuperscript{\textdaggerdbl} & 1.15 \phantom{-} & 0.31 \textsuperscript{\textdagger} & 0.94 \textsuperscript{\textdagger} & 0.86 \phantom{-} & 0.44 \phantom{-} & 0.26 \textsuperscript{\textdagger} & 1.03 \phantom{-} & 0.76 \phantom{-} & 1.07 \phantom{-} & 1.72 \phantom{-} & 1.26 \phantom{-} & 1.67 \phantom{-} & 0.87 \\
DISK SEQ R & -- & -- & 1.03 \phantom{-} & 0.55 \textsuperscript{\textdaggerdbl} & 1.40 \phantom{-} & 1.23 \phantom{-} & 2.62 \phantom{-} & 1.72 \phantom{-} & 1.59 \textsuperscript{\textdaggerdbl} & 0.74 \textsuperscript{\textdaggerdbl} & 0.94 \textsuperscript{\textdaggerdbl} & 1.42 \textsuperscript{\textdaggerdbl} & 1.00 \phantom{-} & 1.32 \phantom{-} & 0.67 \phantom{-} & 1.45 \phantom{-} & 1.11 \\
DISK SEQ W & 1.40 \textsuperscript{\textdagger} & 0.66 \textsuperscript{\textdagger} & 0.64 \textsuperscript{\textdaggerdbl} & 0.65 \textsuperscript{\textdaggerdbl} & 1.88 \phantom{-} & 1.13 \phantom{-} & 0.62 \textsuperscript{\textdagger} & 1.76 \phantom{-} & 1.12 \phantom{-} & 0.55 \phantom{-} & 0.71 \phantom{-} & 0.80 \phantom{-} & 0.92 \phantom{-} & 0.82 \phantom{-} & 1.13 \phantom{-} & 0.91 \phantom{-} & 0.98 \\
DISKB LAT & 1.31 \phantom{-} & 0.56 \phantom{-} & 0.61 \phantom{-} & 1.06 \phantom{-} & 1.46 \phantom{-} & 1.85 \phantom{-} & 1.24 \phantom{-} & 0.78 \phantom{-} & 0.58 \phantom{-} & 1.02 \phantom{-} & 0.35 \phantom{-} & 0.65 \phantom{-} & 0.92 \phantom{-} & 0.64 \phantom{-} & 1.04 \phantom{-} & 0.93 \phantom{-} & 0.94 \\
DISKB THR & 0.77 \phantom{-} & 0.83 \phantom{-} & 0.98 \phantom{-} & 0.70 \phantom{-} & 1.30 \textsuperscript{\textdagger} & 1.05 \textsuperscript{\textdagger} & 0.43 \phantom{-} & 1.40 \phantom{-} & 0.80 \phantom{-} & 0.71 \phantom{-} & 0.99 \phantom{-} & 0.55 \phantom{-} & 0.69 \phantom{-} & 0.42 \textsuperscript{\textdaggerdbl} & 1.27 \textsuperscript{\textdagger} & 0.53 \textsuperscript{\textdaggerdbl} & 0.84 \\
NET 1 & 1.87 \phantom{-} & 5.18 \phantom{-} & 3.48 \phantom{-} & 1.81 \phantom{-} & 1.02 \phantom{-} & 0.76 \phantom{-} & 0.51 \phantom{-} & 1.10 \phantom{-} & 1.37 \phantom{-} & 1.00 \phantom{-} & 1.09 \phantom{-} & 0.88 \phantom{-} & 0.76 \phantom{-} & 1.08 \phantom{-} & 0.75 \phantom{-} & 0.35 \phantom{-} & 1.44 \\
NET 2 & 0.83 \phantom{-} & 0.38 \phantom{-} & 0.67 \phantom{-} & 0.46 \phantom{-} & 1.90 \phantom{-} & 0.79 \phantom{-} & 1.17 \phantom{-} & 2.02 \phantom{-} & 1.28 \phantom{-} & 0.84 \phantom{-} & 1.26 \phantom{-} & 0.75 \phantom{-} & 1.28 \phantom{-} & 1.32 \phantom{-} & 1.11 \phantom{-} & 0.88 \phantom{-} & 1.06 \\
NET 3 & 1.48 \phantom{-} & 0.90 \phantom{-} & 2.77 \phantom{-} & 1.89 \phantom{-} & 0.95 \phantom{-} & 0.45 \phantom{-} & 0.90 \phantom{-} & 0.88 \phantom{-} & 0.74 \phantom{-} & 0.31 \textsuperscript{\textdagger} & 0.60 \phantom{-} & 1.03 \phantom{-} & 0.46 \textsuperscript{\textdagger} & 0.45 \phantom{-} & 0.48 \textsuperscript{\textdagger} & 0.43 \phantom{-} & 0.92 \\
NET 4 & 1.03 \phantom{-} & 1.91 \phantom{-} & 2.30 \phantom{-} & 3.34 \phantom{-} & 0.99 \phantom{-} & 0.56 \phantom{-} & 0.60 \phantom{-} & 1.06 \phantom{-} & 1.25 \phantom{-} & 0.30 \textsuperscript{\textdagger} & 1.85 \phantom{-} & 0.95 \phantom{-} & 0.45 \textsuperscript{\textdagger} & 0.74 \phantom{-} & 0.92 \phantom{-} & 0.50 \textsuperscript{\textdagger} & 1.17 \\
NET 5 & 1.67 \phantom{-} & 2.61 \phantom{-} & 3.20 \phantom{-} & 3.97 \phantom{-} & 0.67 \textsuperscript{\textdaggerdbl} & 0.57 \textsuperscript{\textdaggerdbl} & 0.81 \textsuperscript{\textdagger} & 0.68 \phantom{-} & 0.72 \phantom{-} & 1.05 \phantom{-} & 0.50 \phantom{-} & 0.86 \phantom{-} & 1.81 \phantom{-} & 0.96 \textsuperscript{\textdagger} & 2.65 \phantom{-} & 1.79 \phantom{-} & 1.53 \\
NETB 1 & 1.81 \phantom{-} & 1.26 \phantom{-} & 0.93 \phantom{-} & 0.98 \phantom{-} & 1.10 \phantom{-} & 0.80 \phantom{-} & 0.93 \phantom{-} & 0.96 \phantom{-} & 1.92 \phantom{-} & 1.49 \phantom{-} & 1.56 \phantom{-} & 1.46 \phantom{-} & -- & -- & -- & -- & 0.95 \\
NETB 2 & 1.92 \phantom{-} & 2.56 \phantom{-} & 3.63 \phantom{-} & 1.45 \phantom{-} & 1.02 \phantom{-} & 0.39 \textsuperscript{\textdagger} & 1.01 \phantom{-} & 0.81 \phantom{-} & 1.80 \phantom{-} & 1.27 \phantom{-} & 1.11 \phantom{-} & 1.46 \phantom{-} & 0.84 \phantom{-} & 0.91 \phantom{-} & 0.60 \phantom{-} & 1.13 \phantom{-} & 1.37 \\
APPB & 1.04 \phantom{-} & 0.46 \textsuperscript{\textdagger} & 0.27 \textsuperscript{\textdaggerdbl} & 0.39 \textsuperscript{\textdaggerdbl} & 1.82 \phantom{-} & 0.55 \phantom{-} & 0.56 \textsuperscript{\textdagger} & 1.70 \phantom{-} & 0.38 \textsuperscript{\textdagger} & 0.97 \phantom{-} & 1.12 \textsuperscript{\textdagger} & 0.46 \textsuperscript{\textdagger} & 0.53 \phantom{-} & 0.95 \phantom{-} & 1.31 \phantom{-} & 1.05 \phantom{-} & 0.85 \\
\hline
\textbf{Overall} & 0.10 \phantom{-} & 0.09 \phantom{-} & 0.11 \phantom{-} & 0.10 \phantom{-} & 0.26 \phantom{-} & 0.21 \phantom{-} & 0.14 \phantom{-} & 0.20 \phantom{-} & 0.12 \phantom{-} & 0.09 \phantom{-} & 0.13 \phantom{-} & 0.10 \phantom{-} & 0.10 \phantom{-} & 0.17 \phantom{-} & 0.14 \phantom{-} & 0.12 \phantom{-} & \\ \bottomrule
\end{tabular}
\caption{\nw{Time-series forecasting with VAR model, showing for each resource metric and each VM the corresponding MASE of the prediction. \textsuperscript{\textdagger}: associated MAE < 0.05, \textsuperscript{\textdaggerdbl}: associated MAE < 0.02.}}
\label{tab:forecasting-var}
\end{table*}

\begin{table*}[ht]

\setlength{\tabcolsep}{3.4pt}
\fontsize{8}{9.6}\selectfont
\centering
\begin{tabular}{@{}r|cccc|cccc|cccc|cccc|c@{}}
& \multicolumn{4}{c|}{\textbf{AWS}} & \multicolumn{4}{c|}{\textbf{Azure}} & \multicolumn{4}{c|}{\textbf{GCP}} & \multicolumn{4}{c|}{\textbf{EGI}} & \\ \hline
\textbf{Metric} & C1 & C2 & C3 & C4 & C1 & C2 & C3 & C4 & C1 & C2 & C3 & C4 & C1 & C2 & C3 & C4 & \textbf{Overall} \\ \hline
CPU EVENTS & 0.64 \phantom{-} & 0.76 \phantom{-} & 0.50 \textsuperscript{\textdagger} & 0.44 \textsuperscript{\textdagger} & 1.45 \phantom{-} & 0.97 \phantom{-} & 0.27 \textsuperscript{\textdagger} & 0.75 \phantom{-} & 0.61 \phantom{-} & 0.30 \textsuperscript{\textdagger} & 0.49 \textsuperscript{\textdagger} & 0.23 \textsuperscript{\textdagger} & 0.40 \textsuperscript{\textdagger} & 0.53 \phantom{-} & 0.52 \phantom{-} & 1.39 \phantom{-} & 0.64 \\
CPU LAT & 0.66 \phantom{-} & 0.65 \phantom{-} & 0.73 \phantom{-} & 0.54 \phantom{-} & 1.31 \phantom{-} & 0.94 \phantom{-} & 0.25 \textsuperscript{\textdagger} & 1.12 \phantom{-} & 0.45 \phantom{-} & 0.24 \textsuperscript{\textdaggerdbl} & 0.68 \phantom{-} & 0.22 \textsuperscript{\textdaggerdbl} & 0.67 \phantom{-} & 0.33 \textsuperscript{\textdaggerdbl} & 0.58 \phantom{-} & 4.28 \phantom{-} & 0.85 \\
CPU TH LAT & 0.89 \phantom{-} & 0.40 \textsuperscript{\textdagger} & 0.62 \phantom{-} & 0.72 \phantom{-} & 1.22 \phantom{-} & 0.86 \phantom{-} & 0.93 \phantom{-} & 1.35 \phantom{-} & 1.08 \phantom{-} & 0.53 \phantom{-} & 0.92 \phantom{-} & 0.36 \phantom{-} & 0.47 \textsuperscript{\textdagger} & 0.31 \phantom{-} & 0.84 \phantom{-} & 0.72 \phantom{-} & 0.77 \\
CPU SHA256 & 0.63 \phantom{-} & 0.29 \textsuperscript{\textdagger} & 0.71 \phantom{-} & 0.23 \textsuperscript{\textdaggerdbl} & 1.95 \phantom{-} & 0.89 \phantom{-} & 0.47 \textsuperscript{\textdagger} & 1.68 \phantom{-} & 0.95 \phantom{-} & 0.60 \phantom{-} & 0.37 \phantom{-} & 0.73 \phantom{-} & 0.65 \phantom{-} & 0.98 \phantom{-} & 0.58 \phantom{-} & 0.60 \phantom{-} & 0.77 \\
CPU BZIP2 & 0.54 \textsuperscript{\textdagger} & 0.02 \textsuperscript{\textdaggerdbl} & 0.39 \textsuperscript{\textdaggerdbl} & 0.67 \phantom{-} & 2.06 \phantom{-} & 0.50 \phantom{-} & 0.40 \textsuperscript{\textdagger} & 2.38 \phantom{-} & 0.52 \phantom{-} & 0.65 \phantom{-} & 0.60 \phantom{-} & 1.03 \phantom{-} & 0.93 \phantom{-} & 0.39 \phantom{-} & 1.22 \phantom{-} & 1.30 \phantom{-} & 0.85 \\
CPU AES & 2.11 \phantom{-} & 0.13 \textsuperscript{\textdaggerdbl} & 0.48 \textsuperscript{\textdagger} & 0.41 \textsuperscript{\textdagger} & 1.20 \phantom{-} & 0.58 \phantom{-} & 1.14 \phantom{-} & 1.78 \phantom{-} & 0.48 \textsuperscript{\textdagger} & 1.44 \phantom{-} & 0.75 \phantom{-} & 0.52 \textsuperscript{\textdagger} & 0.52 \phantom{-} & 0.68 \phantom{-} & 0.77 \phantom{-} & 1.42 \phantom{-} & 0.9 \\
CPU DUR & 0.86 \phantom{-} & 0.79 \phantom{-} & 0.54 \phantom{-} & 0.90 \phantom{-} & 0.53 \phantom{-} & 0.60 \phantom{-} & 0.75 \phantom{-} & 1.61 \phantom{-} & 0.73 \phantom{-} & 0.95 \phantom{-} & 0.75 \phantom{-} & 1.06 \phantom{-} & 0.95 \phantom{-} & 0.36 \phantom{-} & 1.02 \phantom{-} & 0.57 \phantom{-} & 0.81 \\
MEM SPEED & 0.26 \textsuperscript{\textdaggerdbl} & 0.26 \textsuperscript{\textdagger} & 0.05 \textsuperscript{\textdaggerdbl} & 0.66 \phantom{-} & 2.12 \phantom{-} & 0.70 \phantom{-} & 1.00 \phantom{-} & 0.71 \phantom{-} & 0.12 \textsuperscript{\textdaggerdbl} & 0.58 \phantom{-} & 0.40 \textsuperscript{\textdaggerdbl} & 0.63 \phantom{-} & 0.43 \phantom{-} & 0.61 \phantom{-} & 0.86 \phantom{-} & 0.67 \phantom{-} & 0.63 \\
MEM LAT & 0.21 \textsuperscript{\textdaggerdbl} & 0.50 \textsuperscript{\textdagger} & 0.09 \textsuperscript{\textdaggerdbl} & 0.37 \phantom{-} & 1.92 \phantom{-} & 0.71 \phantom{-} & 1.12 \phantom{-} & 0.76 \phantom{-} & 0.22 \textsuperscript{\textdaggerdbl} & 1.04 \phantom{-} & 0.10 \textsuperscript{\textdaggerdbl} & 0.44 \phantom{-} & 0.52 \phantom{-} & 0.60 \phantom{-} & 0.76 \phantom{-} & 0.46 \phantom{-} & 0.61 \\
DISK FILE R & 0.47 \phantom{-} & 0.55 \phantom{-} & 0.58 \phantom{-} & 0.86 \phantom{-} & 1.32 \phantom{-} & 0.53 \phantom{-} & 2.91 \phantom{-} & 3.62 \phantom{-} & 0.32 \phantom{-} & 0.18 \textsuperscript{\textdagger} & 1.24 \phantom{-} & 0.67 \phantom{-} & 0.63 \phantom{-} & 1.21 \phantom{-} & 1.16 \phantom{-} & 0.42 \phantom{-} & 1.04 \\
DISK FILE W & 0.47 \phantom{-} & 0.55 \phantom{-} & 0.58 \phantom{-} & 0.86 \phantom{-} & 1.32 \phantom{-} & 0.53 \phantom{-} & 2.91 \phantom{-} & 3.61 \phantom{-} & 0.32 \phantom{-} & 0.18 \textsuperscript{\textdagger} & 1.23 \phantom{-} & 0.67 \phantom{-} & 0.63 \phantom{-} & 1.21 \phantom{-} & 1.16 \phantom{-} & 0.42 \phantom{-} & 1.04 \\
DISK FILE F & 0.47 \phantom{-} & 0.55 \phantom{-} & 0.58 \phantom{-} & 0.86 \phantom{-} & 1.32 \phantom{-} & 0.53 \phantom{-} & 2.91 \phantom{-} & 3.61 \phantom{-} & 0.32 \phantom{-} & 0.18 \textsuperscript{\textdagger} & 1.24 \phantom{-} & 0.67 \phantom{-} & 0.60 \phantom{-} & 1.21 \phantom{-} & 1.16 \phantom{-} & 0.42 \phantom{-} & 1.04 \\
DISK THR R & 0.47 \phantom{-} & 0.55 \phantom{-} & 0.58 \phantom{-} & 0.86 \phantom{-} & 1.32 \phantom{-} & 0.53 \phantom{-} & 2.91 \phantom{-} & 3.61 \phantom{-} & 0.32 \phantom{-} & 0.18 \textsuperscript{\textdagger} & 1.23 \phantom{-} & 0.67 \phantom{-} & 0.62 \phantom{-} & 1.21 \phantom{-} & 1.16 \phantom{-} & 0.42 \phantom{-} & 1.04 \\
DISK THR W & 0.47 \phantom{-} & 0.55 \phantom{-} & 0.58 \phantom{-} & 0.86 \phantom{-} & 1.32 \phantom{-} & 0.53 \phantom{-} & 2.92 \phantom{-} & 3.61 \phantom{-} & 0.32 \phantom{-} & 0.18 \textsuperscript{\textdagger} & 1.24 \phantom{-} & 0.67 \phantom{-} & 0.64 \phantom{-} & 1.21 \phantom{-} & 1.16 \phantom{-} & 0.42 \phantom{-} & 1.04 \\
DISK LAT & 0.76 \phantom{-} & 0.10 \textsuperscript{\textdaggerdbl} & 1.03 \phantom{-} & 0.58 \phantom{-} & 1.31 \phantom{-} & 0.49 \phantom{-} & 3.17 \phantom{-} & 4.49 \phantom{-} & 0.34 \phantom{-} & 0.20 \textsuperscript{\textdagger} & 1.39 \phantom{-} & 0.71 \phantom{-} & 0.45 \textsuperscript{\textdagger} & 1.25 \phantom{-} & 0.86 \phantom{-} & 0.56 \phantom{-} & 1.11 \\
DISK SEEK & -- & -- & 1.06 \textsuperscript{\textdaggerdbl} & 0.16 \textsuperscript{\textdaggerdbl} & 1.02 \phantom{-} & 0.33 \phantom{-} & 0.19 \textsuperscript{\textdaggerdbl} & 0.55 \phantom{-} & 0.49 \phantom{-} & 0.15 \textsuperscript{\textdagger} & 1.14 \phantom{-} & 1.19 \phantom{-} & 1.21 \phantom{-} & 1.62 \phantom{-} & 0.78 \phantom{-} & 1.35 \phantom{-} & 0.7 \\
DISK SEQ R & -- & -- & 1.05 \phantom{-} & 0.31 \textsuperscript{\textdaggerdbl} & 1.13 \phantom{-} & 0.35 \phantom{-} & 1.71 \phantom{-} & 0.85 \phantom{-} & 0.38 \textsuperscript{\textdaggerdbl} & 0.57 \textsuperscript{\textdaggerdbl} & 0.70 \textsuperscript{\textdaggerdbl} & 0.41 \textsuperscript{\textdaggerdbl} & 1.04 \phantom{-} & 1.44 \phantom{-} & 0.77 \phantom{-} & 1.21 \phantom{-} & 0.74 \\
DISK SEQ W & 1.11 \phantom{-} & 0.09 \textsuperscript{\textdaggerdbl} & 0.39 \textsuperscript{\textdaggerdbl} & 0.24 \textsuperscript{\textdaggerdbl} & 1.34 \phantom{-} & 0.29 \textsuperscript{\textdagger} & 0.62 \phantom{-} & 0.81 \textsuperscript{\textdagger} & 0.77 \phantom{-} & 0.50 \phantom{-} & 0.73 \phantom{-} & 0.20 \phantom{-} & 1.14 \phantom{-} & 0.79 \phantom{-} & 1.24 \phantom{-} & 0.52 \phantom{-} & 0.68 \\
DISKB LAT & 1.00 \phantom{-} & 0.63 \phantom{-} & 0.37 \phantom{-} & 0.87 \phantom{-} & 1.11 \phantom{-} & 0.92 \phantom{-} & 1.56 \phantom{-} & 1.33 \phantom{-} & 0.21 \phantom{-} & 0.31 \phantom{-} & 0.31 \phantom{-} & 0.26 \phantom{-} & 1.35 \phantom{-} & 0.46 \phantom{-} & 0.98 \phantom{-} & 0.92 \phantom{-} & 0.79 \\
DISKB THR & 0.63 \phantom{-} & 0.30 \phantom{-} & 1.23 \phantom{-} & 0.61 \phantom{-} & 0.32 \textsuperscript{\textdaggerdbl} & 0.30 \textsuperscript{\textdaggerdbl} & 0.78 \phantom{-} & 1.07 \phantom{-} & 0.60 \phantom{-} & 0.52 \phantom{-} & 0.48 \phantom{-} & 0.57 \phantom{-} & 0.71 \phantom{-} & 0.23 \textsuperscript{\textdaggerdbl} & 0.05 \textsuperscript{\textdaggerdbl} & 0.33 \textsuperscript{\textdaggerdbl} & 0.55 \\
NET 1 & 0.84 \phantom{-} & 2.54 \phantom{-} & 0.97 \phantom{-} & 1.08 \phantom{-} & 0.66 \phantom{-} & 0.84 \phantom{-} & 0.67 \phantom{-} & 1.00 \phantom{-} & 0.26 \textsuperscript{\textdagger} & 0.20 \textsuperscript{\textdagger} & 0.68 \phantom{-} & 0.40 \textsuperscript{\textdagger} & 0.62 \phantom{-} & 0.49 \phantom{-} & 0.47 \phantom{-} & 0.43 \phantom{-} & 0.76 \\
NET 2 & 1.19 \phantom{-} & 0.31 \phantom{-} & 0.57 \phantom{-} & 0.57 \phantom{-} & 0.49 \phantom{-} & 0.41 \phantom{-} & 0.70 \phantom{-} & 0.78 \phantom{-} & 0.53 \phantom{-} & 1.02 \phantom{-} & 0.63 \phantom{-} & 0.90 \phantom{-} & 0.63 \phantom{-} & 0.69 \phantom{-} & 0.71 \phantom{-} & 0.93 \phantom{-} & 0.69 \\
NET 3 & 1.86 \phantom{-} & 1.30 \phantom{-} & 1.45 \phantom{-} & 1.16 \phantom{-} & 0.72 \phantom{-} & 0.53 \phantom{-} & 0.54 \phantom{-} & 0.36 \phantom{-} & 0.55 \phantom{-} & 0.13 \textsuperscript{\textdagger} & 0.19 \textsuperscript{\textdagger} & 0.76 \phantom{-} & 0.73 \phantom{-} & 0.47 \phantom{-} & 0.47 \phantom{-} & 0.41 \phantom{-} & 0.73 \\
NET 4 & 0.77 \phantom{-} & 2.18 \phantom{-} & 1.91 \phantom{-} & 2.13 \phantom{-} & 0.89 \phantom{-} & 0.77 \phantom{-} & 0.64 \phantom{-} & 0.88 \phantom{-} & 1.36 \phantom{-} & 0.21 \textsuperscript{\textdagger} & 1.33 \phantom{-} & 1.19 \phantom{-} & 0.65 \phantom{-} & 0.33 \textsuperscript{\textdagger} & 0.66 \phantom{-} & 0.49 \phantom{-} & 1.02 \\
NET 5 & 2.70 \phantom{-} & 4.13 \phantom{-} & 3.26 \phantom{-} & 3.94 \phantom{-} & 0.48 \textsuperscript{\textdaggerdbl} & 0.44 \textsuperscript{\textdaggerdbl} & 0.37 \textsuperscript{\textdagger} & 0.54 \phantom{-} & 0.62 \phantom{-} & 0.87 \phantom{-} & 0.36 \phantom{-} & 0.43 \phantom{-} & 1.21 \phantom{-} & 0.73 \textsuperscript{\textdagger} & 0.60 \textsuperscript{\textdagger} & 0.97 \textsuperscript{\textdagger} & 1.35 \\
NETB 1 & 0.55 \textsuperscript{\textdagger} & 1.37 \phantom{-} & 0.25 \textsuperscript{\textdagger} & 0.30 \textsuperscript{\textdagger} & 1.73 \phantom{-} & 0.70 \phantom{-} & 0.95 \phantom{-} & 0.48 \phantom{-} & 1.04 \phantom{-} & 0.56 \phantom{-} & 0.55 \phantom{-} & 1.34 \phantom{-} & -- & -- & -- & -- & 0.61 \\
NETB 2 & 0.64 \phantom{-} & 1.44 \phantom{-} & 0.77 \phantom{-} & 0.59 \phantom{-} & 0.97 \phantom{-} & 0.60 \phantom{-} & 0.92 \phantom{-} & 0.87 \phantom{-} & 0.73 \phantom{-} & 0.36 \phantom{-} & 1.03 \phantom{-} & 0.46 \phantom{-} & 0.74 \phantom{-} & 0.50 \phantom{-} & 0.64 \phantom{-} & 1.40 \phantom{-} & 0.79 \\
APPB & 1.47 \phantom{-} & 0.33 \textsuperscript{\textdagger} & 0.05 \textsuperscript{\textdaggerdbl} & 0.14 \textsuperscript{\textdaggerdbl} & 1.75 \phantom{-} & 0.62 \phantom{-} & 0.63 \phantom{-} & 1.23 \phantom{-} & 0.12 \textsuperscript{\textdaggerdbl} & 0.41 \phantom{-} & 1.15 \textsuperscript{\textdagger} & 0.60 \phantom{-} & 0.49 \phantom{-} & 0.51 \phantom{-} & 1.20 \phantom{-} & 0.85 \phantom{-} & 0.72 \\
\hline
\textbf{Overall} & 0.11 \phantom{-} & 0.09 \phantom{-} & 0.10 \phantom{-} & 0.11 \phantom{-} & 0.29 \phantom{-} & 0.14 \phantom{-} & 0.18 \phantom{-} & 0.22 \phantom{-} & 0.10 \phantom{-} & 0.09 \phantom{-} & 0.15 \phantom{-} & 0.13 \phantom{-} & 0.13 \phantom{-} & 0.17 \phantom{-} & 0.20 \phantom{-} & 0.16 \phantom{-} & \\ \bottomrule
\end{tabular}
\caption{\nw{Time-series forecasting with SARIMAX model, showing for each resource metric and each VM the corresponding MASE of the prediction. \textsuperscript{\textdagger}: associated MAE < 0.05, \textsuperscript{\textdaggerdbl}: associated MAE < 0.02.}}
\label{tab:forecasting-sarimax}
\end{table*}
